# Supplementary material for: Efficient Sketching Algorithm for Sparse Binary Data
Source: arXiv:1910.04658 source file (2019-10-10)
Supplement: Supplementary file 1 [file appendix_plots.tex]

\newpage
\section{Extended Experimental Results}
\begin{figure}[ht]
\centering
\includegraphics[height=7.2cm,width=16.5cm]{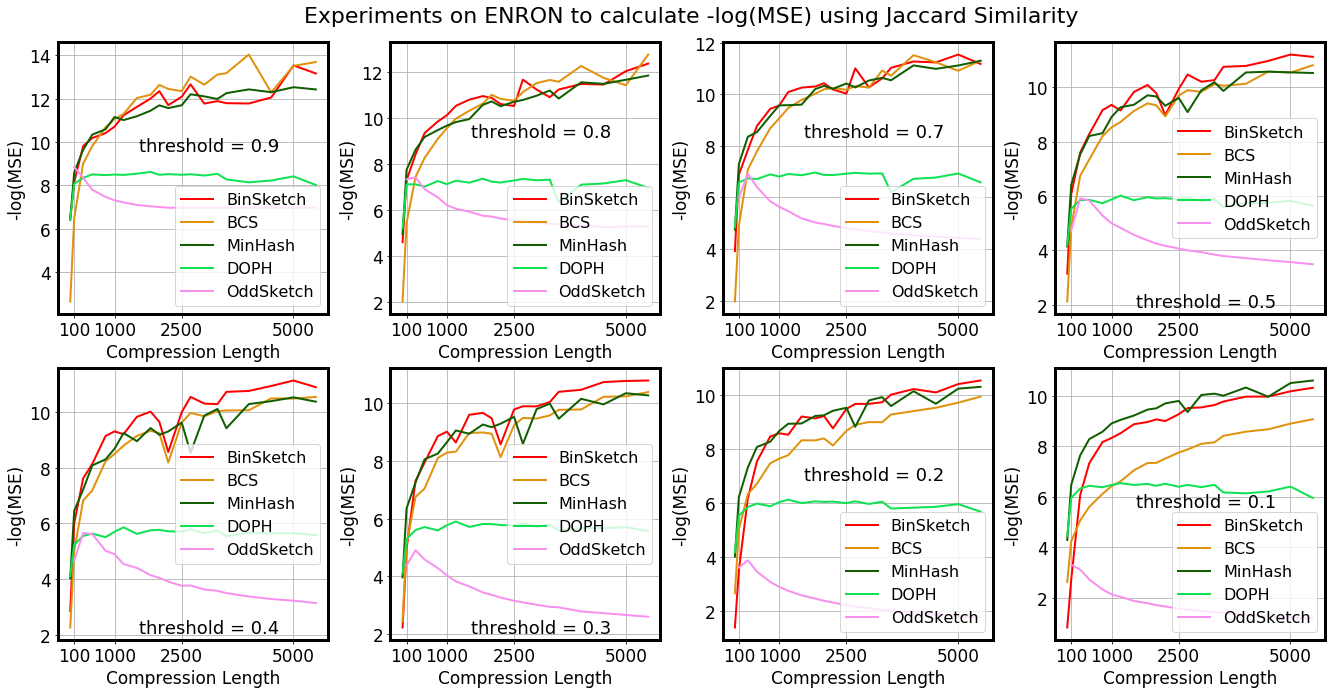}
\includegraphics[height=7.2cm,width=16.5cm]{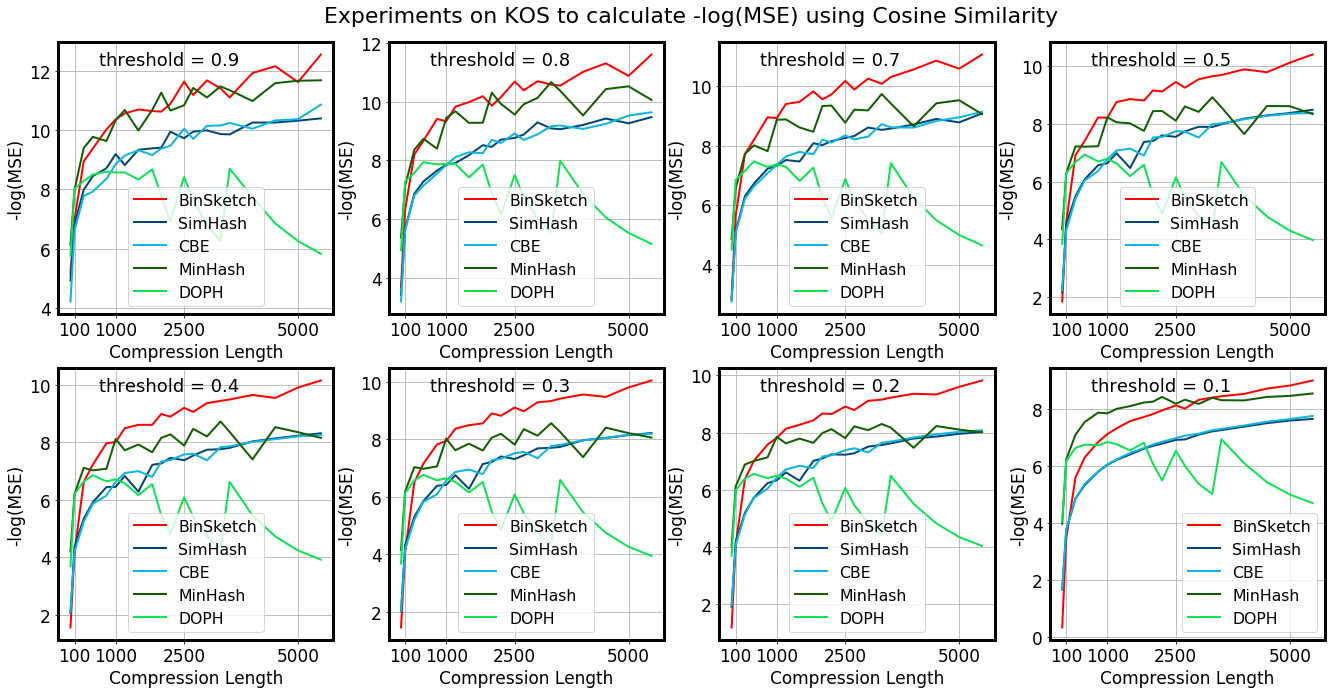}
\includegraphics[height=7.2cm,width=16.5cm]{MSE_JS_KOS.png}
   \vspace*{-0.3cm}
\caption{Comparison of $-\log(\MSE)$ measure on ENRON and KOS datasets.}
\label{fig:Accuracy}
\end{figure}

\begin{figure*}[ht!]
\centering
\includegraphics[height=8cm,width=16.5cm]{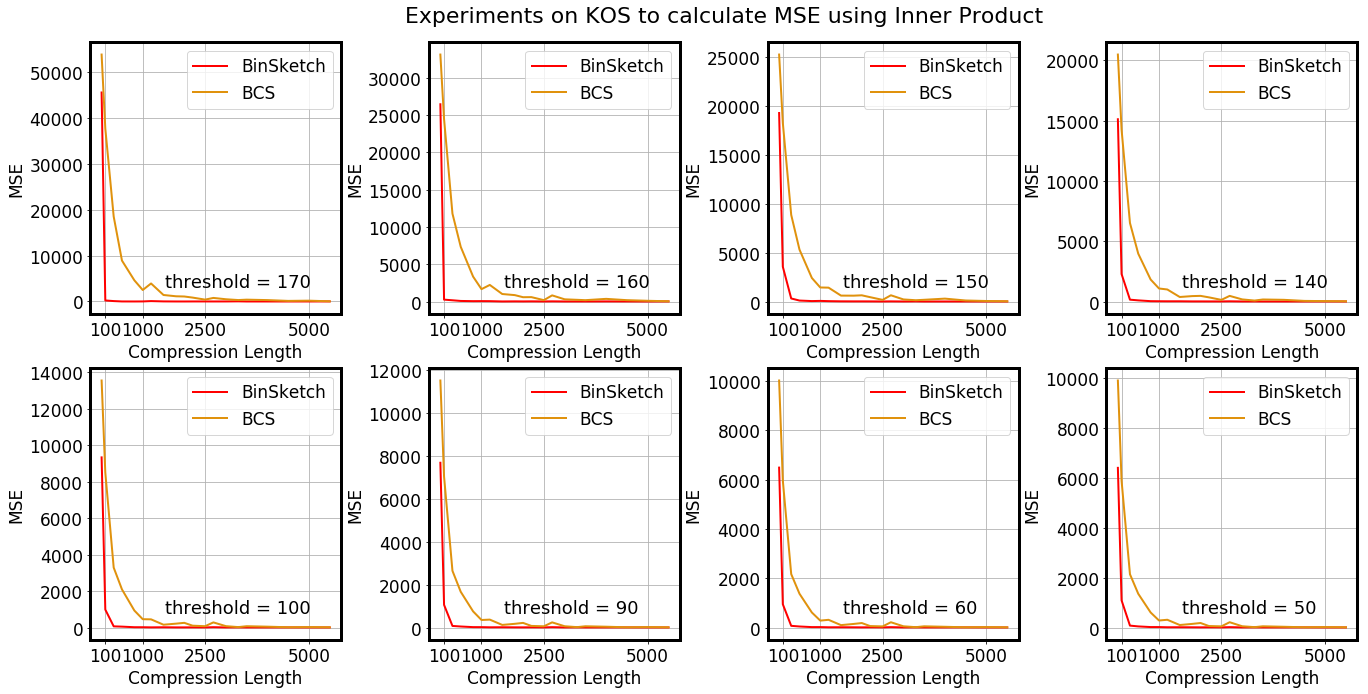}
\includegraphics[height=8cm,width=16.5cm]{Ranking_CS_Precision_ENRON.png}
\includegraphics[height=8cm,width=16.5cm]{Ranking_CS_Recall_ENRON.png}
   \vspace*{-0.3cm}
\caption{\small{Comparison of $\MSE$   on KOS dataset for Inner Product, and comparison of Precision and Recall   on ENRON dataset for Cosine Similarity.}}
\label{fig:Accuracy}
\end{figure*}

\begin{figure*}[ht!]
\centering
\includegraphics[height=8cm,width=16.5cm]{Ranking_CS_Accuracy_KOS.png}
\includegraphics[height=8cm,width=16.5cm]{Ranking_CS_Precision_KOS.png}
\includegraphics[height=8cm,width=16.5cm]{Ranking_CS_Recall_ENRON.png}
   \vspace*{-0.3cm}
\caption{Comparison of Accuracy, Precision, Recall measure on  KOS datasets for Cosine Similarity.}
\label{fig:Accuracy}
\end{figure*}

\begin{figure*}[ht!]
\centering
\includegraphics[height=8cm,width=16.5cm]{Ranking_CS_Accuracy_BBC.png}
\includegraphics[height=8cm,width=16.5cm]{Ranking_CS_Precision_BBC.png}
\includegraphics[height=8cm,width=16.5cm]{Ranking_CS_Recall_BBC.png}
   \vspace*{-0.3cm}
\caption{Comparison of Accuracy, Precision, Recall measure on  BBC datasets for Cosine Similarity.}
\label{fig:Accuracy}
\end{figure*}

\begin{figure*}[ht!]
\centering
\includegraphics[height=8cm,width=16.5cm]{Ranking_JS_Accuracy_BBC.png}
\includegraphics[height=8cm,width=16.5cm]{Ranking_JS_Precision_BBC.png}
\includegraphics[height=8cm,width=16.5cm]{Ranking_JS_Recall_BBC.png}
   \vspace*{-0.3cm}
\caption{Comparison of Accuracy, Precision, Recall measure on  BBC datasets for Jaccard Similarity.}
\label{fig:Accuracy}
\end{figure*}

\begin{figure*}[ht!]
\centering
\includegraphics[height=8cm,width=16.5cm]{Ranking_JS_Accuracy_KOS.png}
\includegraphics[height=8cm,width=16.5cm]{Ranking_JS_Precision_KOS.png}
\includegraphics[height=8cm,width=16.5cm]{Ranking_JS_Recall_KOS.png}
   \vspace*{-0.3cm}
\caption{Comparison of Accuracy, Precision, Recall measure on  KOS datasets for Jaccard Similarity.}
\label{fig:Accuracy}
\end{figure*}

\begin{figure*}[ht!]
\centering
\includegraphics[height=8cm,width=16.5cm]{Ranking_JS_Precision_NYTimes.png}
\includegraphics[height=8cm,width=16.5cm]{Ranking_JS_Recall_NYTimes.png}
\includegraphics[height=8cm,width=16.5cm]{Ranking_JS_Precision_ENRON.png}
   \vspace*{-0.3cm}
\caption{Comparison of   Precision, Recall   on  NYTimes and Precision on ENRON datasets for Jaccard Similarity.}
\label{fig:Accuracy}
\end{figure*}

\begin{figure*}[ht!]
\centering
\includegraphics[height=8cm,width=16.5cm]{Ranking_IP_Accuracy_NYTimes.png}
\includegraphics[height=8cm,width=16.5cm]{Ranking_IP_Precision_NYTimes.png}
\includegraphics[height=8cm,width=16.5cm]{Ranking_IP_Recall_NYTimes.png}
   \vspace*{-0.3cm}
\caption{Comparison of Accuracy, Precision, Recall measure on  NYTimes datasets for Inner Product.}
\label{fig:Accuracy}
\end{figure*}

\begin{figure*}[ht!]
\centering
\includegraphics[height=8cm,width=16.5cm]{Ranking_JS_Recall_ENRON.png}
\includegraphics[height=8cm,width=16.5cm]{Ranking_IP_Recall_ENRON.png}
\includegraphics[height=8cm,width=16.5cm]{Ranking_IP_Recall_KOS.png}
   \vspace*{-0.3cm}
\caption{Comparison of  Recall measure on  ENRON for Jaccard Similarity and ENRON and KOS for Inner Product.}
\label{fig:Accuracy}
\end{figure*}
